# Supplementary material for: Distributed Interview Selection for Stable Matching in Large Random Markets
Source: arXiv:2506.19345 source file (2025-06-24)
Supplement: Supplementary file 2 [file old-appendix.tex]

\begin{proof}(Of Claim \Cref{clm::qtilde-bound-for-hosp-doc-int}.)
We prove the result by an induction from the leaves to the root of tree $T$.

Recall that $p(h,v)$ denotes the residual probability of $h$ at node $v$,
and let $p_1\le p_2\le p_{s-x-y}$ be the $s-x-y$ smallest residual probabilities being used to calculate $\tilde{q}(v)$; the hospitals that have already proposed to $h$ are excluded.

\smallskip\noindent
\emph{Base case: a leaf node}\\
At a leaf node $v$ all the random decisions have been made, so either $d$ has received the desired proposal or not. Therefore $q(v)=\tilde{q}(v)$.


\smallskip\noindent
\emph{Inductive step at internal node $v$}\\
Let $h$ be the hospital making a random choice at node $v$.
Recall that $d$ has received $x$ real and $y$ imaginary proposals prior to reaching node $v$.
Then $\qtilde(v)$ is calculated using $s-x-y$ residual probabilities,
and for each child $u$ of $v$, $\qtilde(u)$ is calculated using $s-x-y$ residual probabilities, with the exception of the children $\overline{u}_{\rl}$ corresponding to a real proposal to doctor $d$ and
$\overline{u}_{\im}$ corresponding to an imaginary proposal to $d$.
$\overline{u}_{\rl}$ and $\overline{u}_{\im}$ are calculated using $s-x-y-1$ residual probabilities,
as in both cases, $h$ makes no further proposals in the run of the double-cut DA.
Finally, in the calculation of $\qtilde(u)$, for $u\ne \overline{u}_{\rl},\overline{u}_{\im}$, all the residual probabilities except at most one are unchanged; the only one that may change is due to the fact that $p(h,u)<p(h,v)$. 

Let $p_u$ be the probability that the edge from $v$ to its child $u$ is chosen when at node $v$.
Then $q(v) = \sum_{\text{$u$ a child of $v$}} p_u \cdot q(u)$.
To prove our inductive bound it will suffice to show that
\begin{align} %\label{eqn::qtilde-bound}
    \qtilde(v) \ge \sum_{\text{$u$ a child of $v$}} p_u \cdot \qtilde(u).
\end{align}

\smallskip\noindent
\emph{Case 1.} $p(h,v)$ is among the smallest $s-x-y$ residual probabilities at node $v$, and $p(h,u)$ is among the smallest $s-x-y$ residual probabilities at each child $u\ne \overline{u}_{rl},\overline{u}_{im}$ of $v$.\\
In this case, we show that \eqref{eqn::qtilde-bound} holds with equality.
To do this we consider the random choices that are made in evaluating $\qtilde(v)$,
by instantiating exactly the randomness needed to select a child $u$ of $v$.

One way to make these random choices is to determine if $h$'s utility for
$d$ equals the utility at node $v$; if so, a further random choice determines if the
proposal is real or imaginary.
At each child, we then make the remaining random choices to determine the probability
of no high real proposal to $d$. But at each node $u$, this probability
is exactly $\qtilde(u)$, for we are using the same random variables apart from the
partially instantiated $p(h,v)$, whose completed instantiation is given by $p(h,u)$ at all nodes $u$ other than $\overline{u}_{rl},\overline{u}_{im}$, where this value is not being used.
Thus $\qtilde(v)=\sum_{\text{$u$ a child of $v$}} p_u\cdot \qtilde(u)$ in this case.

\smallskip\noindent
\emph{Case 2}.  $p(h,v)$ is not among the smallest $s-x-y$ residual probabilities at node $v$, but for the children $u\ne \overline{u}_{\rl},\overline{u}_{\im}$ of $v$, $p(h,u)$ is among the smallest $s-x-y$ residual probabilities at $u$.\\
We use a reduction. We increase $p_{s-x-y}$ until it is equal to $p(h,v)$.
This leaves $\qtilde(u)$ unchanged for all children $u$ of $v$, but reduces the value of $\qtilde(v)$.
When $p_{s-x-y}=p(h,v)$, this becomes Case 1 and \eqref{eqn::qtilde-bound} holds.
Therefore it holds with the original value of $p_{s-x-y}$ too, as the right hand side of \eqref{eqn::qtilde-bound} is unchanged, but the left hand side is increased.

\smallskip\noindent
\emph{Case 3}.  $p(h,v)$ is not among the smallest $s-x-y$ residual probabilities at node $v$, and $p(h,u)$ is not among the smallest $s-x-y$ residual probabilities at any child $u\ne \overline{u}_{rl},\overline{u}_{im}$ of $v$.\\
At every child $u\ne \overline{u}_{rl},\overline{u}_{im}$ of $v$, $\qtilde(u)=\qtilde(v)$, as these probabilities are being computed using the same residual probabilities,
and the probability distribution for selecting a hospitals in $S(u)$ and $S(v)$ are the same as $S(u)=S(v)$.

Let's remove all the terms corresponding to these nodes from \eqref{eqn::qtilde-bound}; it reduces to
%
\begin{align*}
     p_{\overline{u}_{\rl}}\cdot \qtilde(v) + p_{\overline{u}_{\im}}\cdot \qtilde(v)\ge  p_{\overline{u}_{\rl}}\cdot \qtilde(\overline{u}_{\rl}) + p_{\overline{u}_{\im}}\cdot \qtilde(\overline{u}_{\im}).
\end{align*}

We modify this reduced problem as follows: simply increase $p_{s-x-y}$ until it is equal to $p(h,v)$.
This leaves $\qtilde(\overline{u}_{\rl})$ and $\qtilde(\overline{u}_{\im})$ unchanged, but
reduces $\qtilde(v)$. Furthermore, when $p_{s-x-y}=p(h,v)$, we have an instance of Case 1, and
so at this point \eqref{eqn::qtilde-bound} holds, and therefore it also holds prior to the increase in value for $p_{s-x-y}$.
\end{proof}


\begin{proof} (Of \Cref{lem::one-woman-prop-bound}.)
We prove this bound holds regardless of the interview values of the men for women other than $w$, and the private and interview values of the women other than $w$ for all the men. So let's fix all these values. We start by eliminating the zero probability events that a woman has the same utility for any two men. Clearly, these zero probability events are not going to affect our final bound on the probability that $m$ receives no proposal.

It will be helpful to define a tree $T$ which will represent the possible computations of the double-cut DA. 
These computations depend only on $m$'s interview values and on the private and interview values of the women for $m$.
Each random choice of these values defines a computation path. To make these paths unique, whenever two or more men could make a proposal, we let the one with lower rank proceed.

There will be two types of nodes in $T$. Those that correspond to proposals made to women other than $w$, and those that correspond to possible proposals to $w$, which depend on the random choices of the interview values for $w$.
Note that the first type of node represent actions that are fully determined, as both the interview values for these women and the private and interview values of these women are already fixed. Each node of the second type will cover a limited range of utility values for a single man, and it can have three outcomes corresponding to the three edges that will descend from the node: one edge corresponds to a proposal to $w$ with utility in the specified range, the others to there being no proposal to $w$ with a utility in this range: the second edge corresponds to the situation where the interview value would be in the right range for a proposal to $w$,
but $w$'s private value for $m$ wasn't large enough to enable an edge $(w,m)$ to be present, and the third edge corresponds
to $m$'s interview value for $w$ being too small.

Let's make this more precise.
Consider the actions of a single man $m$. Suppose $m$'s utilities for the women other than $w$, which are above the cut at $c(w)=r(w)-\alpha$, are $u_1>u_2>\ldots>u_t$. On each computation path $P$, there will be a subsequence of up to $2t$ nodes corresponding to $m$'s actions. Let $x_1,x_2,\ldots,x_q$ be the type 1 nodes in this subsequence, in the order in which they appear along $P$.
$x_i$ corresponds to the proposal that provides $m$ utility $u_i$. 
To identify the type 2 nodes,
suppose that $u_h\ge r(m)+2> u_{h+1}$ (if either of these is missing, we take $u_0=r(m)+2$ and $u_{t+1}=r(m)+2-\alpha$). We introduce additional nodes $y_{h+1},y_{h+2},\ldots, y_{q}$; $y_i$ has three children, one corresponding
to $m$ making a proposal to $w$ with utility in the range $(u_{i+1},u_i)$, and the other two corresponding to not making a proposal to $w$ with utility in this range. Note that on the path on which $y_i$ made a proposal to $w$ with utility in the range
$(u_i,u_{i+1})$, this is the last action taken by $m$ in this run of the double cut DA, i.e.\ in the computations in the subtree rooted at the relevant child.

On each path $P$, the nodes $x_i$ over all the men $m$ participating in the double-cut DA are arranged in the order in which they would occur in the corresponding run of the double-cut DA. Each node $y_i$ is placed immediately above the corresponding $x_i$.

We now want to upper bound the probability that $w$ receives at most $r$ proposals from the computation continuing from each node $v$ in the tree $T$, which we will do by means of a bottom-up inductive argument on the tree $T$.
To this end, we define the residual proposing probability for man $w$ at a node $v$ who has not yet proposed
to $w$ as follows:
his residual probability, $p(w,v)$, is given by the probability that he has an edge to $w$ providing utility
in the range $(c(w),u)$,
where the nearest type 2 node for node $w$ above $v$ had utility range $(u,u')$, and if there is no such
node, the range is given by $(c(w),r(w)+2)$. 

Suppose there have been $x = x(v)$ proposals to $w$ on the path to $v$,
Let $p_1\le p_2\le \ldots \le p_{s-x}$ be the $s-x$ smallest residual probabilities at node $v$.
Suppose $r>x$, and suppose there are $s-x$ independent attempts to propose to $w$ with respective
probabilities $p_1,p_2,\ldots,p_{s-x}$. Let $\tilde{q}(v)$ be the probability that these attempted proposals yield
at most $r$ actual proposals. If $r\le x$, we define $\tilde{q}(v)=0$.
Let $q(v)$ be the probability that in the subtree rooted at $v$ at most $r-x$ proposals to $w$ are made if $r>x$, and otherwise $q(v)=0$.
 

\begin{claim}\label{clm::indpt-is-worst-manDA}
For every node $v$ in $T$, $q(v)\le \tilde{q}(v)$.
\end{claim}
\begin{proof}
We prove this result by induction.

\smallskip\noindent
\emph{Base case}: A leaf node.\\
If there have been more than $r$ proposals to $w$, then $q(v)=\tilde{q}(v)=0$.
If there had been $x\le r$ proposals, as there are at least $s$ surplus men, at least $s-x$ of them can still propose to $w$ with their residual probability, and these are all independent actions.
Suppose these residual probabilities are $q_1\le q_2\le\ldots\le q_{s-x}$.
These $s-x$ attempted proposals result in a probability $q\ge q(v)$ of at most $r-x$ additional proposals to $w$, as in the actual computation leading to this leaf there may be more that $s$ surplus men, which potentially causes more proposals to $w$.
Attempting to propose with the $s-x$ smallest residual probabilities, $p_1\le p_2\le \ldots \le p_{s-x}$,
yields a probability $\tilde{q}(v)$ of at most $r-x$ additional proposals to $w$, and as these are the smallest
residual probabilities, $\tilde{q}(v)\ge q\ge q(v)$.

\smallskip\noindent
\emph{Inductive step}.
\\
\emph{Case 1}.  A node $v$ with a single child $v'$.\\
Clearly, $q(v)=q(v')$ and $\tilde{q}(v)= \tilde{q}(v')$. So the result holds at node $v$ given it holds at $v'$.

\smallskip\noindent
\emph{Case 2.} A node $v$ with children $\vl$, $\vm$, and $\vr$.\\
Let $m$ be the man choosing whether to propose to $w$ at node $v$, and suppose $\vl$ is the node reached
if she makes this proposal. Suppose further that the edge to $\vl$ is taken with probability $\delta\cdot\tau$, the
edge to $\vr$ with probability $(1-\delta)$, and the edge to $\vm$ with probability $\delta\cdot(1-\tau)$.
Clearly, $q(v)= \delta\cdot\tau\cdot q(\vl) + \delta\cdot(1-\tau)\cdot q(\vm) + (1-\delta)\cdot  q(\vr)$.
We now show that $\tilde{q}(v)\ge \delta\cdot\tau\cdot \tilde{q}(\vl) +  \delta\cdot(1-\tau)\cdot \tilde{q}(\vm) + (1-\delta)\cdot \tilde{q}(\vr)$, and therefore by induction, $\tilde{q}(v) \ge \delta\cdot\tau\cdot q(\vl)+ \delta\cdot(1-\tau) \cdot q+ (\vm) + (1-\delta)\cdot q(\vr) = q(v)$.

Recall that $p_1(v)\le p_2(v)\le\ldots\le p_{s-x}(v)$ are the $s-x$ smallest residual probabilities which are used to evaluate $\tilde{q}(v)$, and similarly $p_1(\vr)\le p_2(\vr)\le\ldots\le p_{s-x}(\vr)$ are the $s-x$ smallest residual probabilities which are used to evaluate $\tilde{q}(\vr)$.

\smallskip\noindent
Case 2.1.  $\{p_1(\vr),p_2(\vr),\ldots,p_{s-x}(\vr)\}$ includes the residual probability $p(w,\vr)$ for $w$ at node $\vr$.\\
Case 2.1.1. $\{p_1(v),p_2(v),\ldots,p_{s-x}(v)\}$ includes the residual probability $p(w,v)$ for $w$ at node $v$.\\
One way to calculate $\tilde{q}(v)$ is to determine whether $w$ proposes to $m$ in two steps:
first, with probability $\delta$, we decide if $w$'s private value for $m$ is in the range that causes a move to one of $\vl$ or $\vm$; then, with a further probability $\tau$ whether to go to $\vl$, and with probability $(1-\tau)$ to $\vm$;
the residual probabilities $\{p_1(v),p_2(v),\ldots,p_{s-x}(v)\}\setminus\{p(w,v\}$ are used to compute both $\tilde{q}(\vl)$ and $\tilde{q}(\vm)$.
While for the move to $\vr$, the residual probabilities $p_1(v),p_2(v),\ldots,p_{s-x}(v)$, with $p(w,v)$ replaced by
$p(w,\vr)$, are used to compute $\tilde{q}(\vr)$; but $p(w,\vr)$ is the probability that $w$ has a proposal to $m$ after the possible range for its private value has been reduced by the range that enabled a move to $\vl$ or $\vm$.

These residual probabilities yield proposing probabilities
$\tilde{q}(\vl)$, $\tilde{q}(\vm)$, and $\tilde{q}(\vr)$ at nodes
$\vl$, $\vm$, and $\vr$, respectively; since these nodes are reached with probabilities $\delta\tau$, $\delta(1-\tau)$, and $1-\delta$,
the resulting probability $\tilde{q}(v)$ at node $v$ therefore equals $\delta\cdot \tau\cdot \tilde{q}(\vl)+ \delta\cdot (1-\tau)\cdot \tilde{q}(\vm) + (1-\delta)\tilde{q}(\vr)$.

\smallskip\noindent
Case 2.1.2.  $\{p_1(v),p_2(v),\ldots,p_{s-x}(v)\}$ does not include the residual probability $p(w,v)$ for $w$ at node $v$.\\
We reduce this case to case 2.1.1 as follows. Suppose we increased $p_{s-x}(v)$ so that it became larger than $p(w,v)$.
Then this setting would become an instance of case 2.1.1, and the modified $\tilde{q}(v)$, would equal 
$\delta\cdot \tau \cdot \tilde{q}(\vl) + \delta\cdot (1-\tau) \cdot \tilde{q}(\vm) + (1-\delta)\tilde{q}(\vr)$.
Now consider reducing $p_{s-x}$ to its actual value; the effect on the probability of at most $r-x$ proposals is only to increase it, as the only change is for one of the proposal attempts to occur with reduced probability.
Therefore $\tilde{q}(v)\ge \delta \tau \tilde{q}(\vl) + \delta\cdot (1-\tau) \cdot \tilde{q}(\vm)+ (1-\delta) \tilde{q}(\vr)$, in this case too.

\smallskip\noindent
Case 2.2.  $\{p_1(\vr),p_2(\vr),\ldots,p_{s-x}(\vr)\}$ does not include the residual probability $p(w,\vr)$ for $w$ at node $\vr$.\\
Then $\{p_1(v),p_2(v),\ldots,p_{s-x}(v)\}$ does not include the residual probability $p(w,v)$ for $w$ at node $v$,
as $p(w,\vr) < p(w,v)$.

We reduce Case 2.2 to Case 2.1.2, as follows.
Imagine reducing both $p(w,\vr)$ and $p(w,v)$ so as to maintain the $\delta$ to $(1-\delta)$ probability split
between choosing to move to one or $\vl$ or $\vm$ and to $\vr$, stopping when
$p(w,\vr)$ is reduced to $p_{s-x}$. This leaves $\tilde{q}(v)$ unchanged, so the bound from case 2.1.2 applies.

\smallskip\noindent
By induction, in every subcase, $\tilde{q}(v)\ge \delta\cdot\tau\cdot \tilde{q}(\vl) + \delta\cdot(1-\tau)\cdot \tilde{q}(\vm) + (1-\delta)\tilde{q}(\vr)$, and therefore, $\tilde{q}(v) \ge \delta\cdot\tau\cdot q(\vl) + delta\cdot(1-\tau)\cdot q(\vm) + (1-\delta)q(\vr) = q(v)$.
\end{proof}

The overall result follows by applying the claim to the root of $T$.
\end{proof}

\begin{proof} (Of \Cref{lem::prob-bound-interval-mismatch-women}.)
We begin by excluding the low probability case that the number of women in $I$ is less than half the expectation or more than twice the expectation. By \Cref{lem::no-BJ}, the failure probability is at most $2/n^{c+2}$.

We will run the man-proposing double-cut DA with a cut at utility $l+1-\sigma$, and at any proposal to a woman in $I$.
But we also prevent a few men from participating at all.
Specifically, we eliminate all men that have an edge to a woman in $I$ with utility in the range $(l+1,l+d+1)$, and all men that have two or more proposals to women in $I$. This ensures that if there is a proposal with utility $x$ to a woman in $I$, it could be to any woman in $I$. What this means is that we can view a proposal to a woman in $I$ as a proposal to the whole set, and handle it in a way that treats the proposal as being equally likely to be to any woman in $I$.
This then allows us to use a lower bound on the number of proposals by these men to women in $I$ to deduce an upper bound on the number of unmatched women in $I$ (both of these statements will be with high probability).

The expected number of men eliminated for having a utility in the range $(l+1,l+d+1)$ is the product of the following terms:
\begin{itemize}
\item 
the number of men in-cone for all the women in the interval $I$, which is the number of men contained in the public rating interval $[l+d-a\alpha,l+a\alpha]$,
which, by \Cref{lem::no-BI}, is at most $(2a+1)\alpha n$ with failure probability at most $1/n^{c+2}$, 
\item 
the number of women in the public rating interval $[l,l+d]$,
which, by \Cref{lem::no-BJ} is at most $2dn$ with failure probability at most $1/n^{c+2}$,
\item 
the probability that there is an edge between a specified man and woman, namely
$k/2a\alpha n$, 
\item
the probability $d$ that the interview increment to the utility ensures an overall utility in the range $(l+1,l+d+1)$,
\end{itemize}
namely,
\begin{align*}
    (2a+1)\alpha n \cdot 2dn\cdot \frac{k}{2a\alpha n} \cdot d
    &= \frac {4(2a+1)}{2a}d^2n
    \le 5(c+2)^2 e^{2\beta k}\ln^2 n,
\end{align*}
as $a\ge 4$.
This brings the running total on the failure probability to $4/n^{c+2}$.

By a Chernoff bound, the number of men eliminated is at most
$10(c+2)^2 e^{2\beta k}\ln^2 n$,
with failure probability $\exp(-5(c+2)^2 e^{2\beta k}\ln^2 n/3) \le 1/n^{c+2}$, if
$(c+2) e^{2\beta k}\ln n\ge \tfrac 35$, which holds as $\beta k > 0$.
Now the running total on the failure probability is $5/n^{c+2}$.

The number of men eliminated for having two proposals into $I$ is at most the number of men in-cone for all the women in the interval, times the number of choices of pairs of women in the interval,
which, by \Cref{lem::no-BJ} is at most $(2dn)^2$ (note the failure probability for this event was counted in the itemized list above), times the probability that there are edges from any one man to both these women, namely,
$(k/2a\alpha n)^2$, yielding the following bound on this number:
\begin{align*}
  (2a+1)\alpha n \cdot \frac{(dn)^2}{2} \cdot \Big(\frac{k}{2a\alpha n}\Big)^2
  &\le \frac{(2a+1)k^2d^2n}{\alpha}\\
  & \le \frac{(2a+1)k^2 (c+2)^2e^{2\beta k}\ln^2 n}{\alpha n}
  \le 1,
\end{align*}
if $n\ge (c+2)^2(2a+1)k^2 e^{2\beta k}\ln^2 n/\alpha$.
Therefore, by a Chernoff bound, at most $(\ln (c+2) n)/\ln 2$ men are eliminated, with failure probability $1/n^{c+2}$.
Now the running total on the failure probability is $6/n^{c+2}$.

As we show in \Cref{lem::prob-bound-interval-mismatch},
the number of unmatched men in each interval of rating length $d$ is at most $2g e^{-\beta k}$ with failure probability
$1/n^{c+2}$. So above the intersection of the cones for the women in $I$, the number of unmatched men is at most
$2ne^{-\beta k}$ with probability at most $1/n^{c+1}$.
Now the running total on the failure probability is $6/n^{c+2}+1/n^{c+1}$.

Therefore the surplus $s$ is at least the number of men in or above the cones for all women in $I$,
i.e.\ with public rating at least $l+d-a\alpha$, which is at least $[1-l-d+(a-1)\alpha]n$,
minus the number of women above the cut, namely those with
public rating at least $l-\sigma$, which is at most $[1-l+\sigma +\alpha]n$ women, minus the number of unmatched men above the cones for all women in $I$,
minus the number of eliminated men.
This is lower bounded by
\begin{align*}
&\big[1-l-d+(a-1)\alpha - (1-l+\sigma+\alpha) - 2e^{-\beta k}\big]n - 2(c+2)^2 e^{2\beta k}\ln^2 n -(\ln (c+2) n)/\ln 2 +g\\
&~~~~\ge (a-3)\alpha n \ge  \alpha n,
\end{align*}
if  $a\ge 4$, $d\le \alpha/4$, $\sigma \le \alpha/4$, $2e^{-\beta k}\le \alpha/4$, $2(c+2)^2 e^{2\beta k}\ln^2 n\le \alpha n/4$, and $g\ge (\ln (c+2) n)/\ln 2$; 
the fourth condition is satisfied as $n\ge (c+2)^2(2a+1)k^2 e^{2\beta k}\ln^2 n/\alpha$ and $a\ge 4$, and
the last condition is satisfied
if $\tfrac 12(c+2)e^{\beta k}\ln n \ge (\ln (c+2) n)/\ln 2$, which is satisfied if $n \ge c+2$, and
$\tfrac 14 \ln 2\cdot (c+2)\cdot e^{\beta k}\ge 1$, which holds as $\beta k\ge 2$.

Now the bound from \Cref{lem::one-woman-prop-bound} applies with I replacing the single woman $w$.
The expected number of proposals to $I$ is calculated as follows:
an edge from a man $m$ is present with probability $\tau=k/2a\alpha n$ and
it is used if its utility is in the range $(l+1-\sigma, l+1)$; note that for each possible private value, there is a probability $\sigma$ that the interview value yields a utility in this range, which gives a probability of $\tau\cdot \sigma$. But the overall probability has to be reduced to account for the possibility of
two or more such edges from $w$ into $I$, which occurs with probability
\begin{align*}
\sum_{i\ge 2} i\cdot {g \choose i} (\tau\sigma)^i \le \sum_{i\ge 2}(g\tau\sigma)\frac{(g\tau\sigma)^{i-1}}{i-1} \le g\tau\sigma e^{g\tau\sigma}\le \tfrac 32 g\tau\sigma, 
\end{align*}
if $e^{g\tau\sigma}\le \tfrac 32$.
Then the expected number of edges is at least $\tfrac12 sg\tau\sigma$.
Now,
\begin{align*}
\frac 12 sg\tau\sigma &\ge \frac a4 \alpha n \cdot g \cdot \frac {k}{4a\alpha n}\cdot \sigma
\ge \frac{kg\sigma}{8}.
\end{align*}
By \Cref{lem::one-man-prop-bound}, applying a Chernoff bound, 
shows that the number of proposals is at least $r=\tfrac{kg\sigma}{16}$ with failure probability at most
$p(s,r)=\exp(-kg\sigma/128)\le \exp(-ke^{\beta k}\sigma(c+2)\ln n/128)\le n^{-(c+2)}$, if $k\cdot e^{\beta k}\sigma\ge 128$.
Now the running total on the failure probability is $7/n^{c+2}+1/n^{c+1}$.

As the proposals into $I$ that we are considering are uniform over $I$, this amounts to a balls and bins problem.
The question we are asking is how many bins remain empty. In expectation, a bin is empty (i.e.\ a woman is unmatched)
with probability at most $e^{-k\sigma/16}$, and so in expectation, at most $ge^{-k\sigma/16}$ bins are empty.
Now, as the indicator variables for whether a bin is empty are negatively correlated, we can apply Chernoff bounds
to this setting, and therefore at most $2ge^{-k\sigma/16}$ bins are empty with failure probability at most
$\exp(-2ge^{-k\sigma/16}/3)\le n^{-(c+2)}$, if $e^{\beta k} e^{-k\sigma/16} \ge 3$.
Now the running total on the failure probability is $8/n^{c+2}+1/n^{c+1}$.
\end{proof}
